# Supplementary material for: Local persistence exponent and its log-periodic oscillations
Source: arXiv:2507.08628 source file (2025-07-11)
Supplement: Supplementary file 1 [file appendix_old.tex]

\appendix
\section{Computation of area-based variables}
\label{sec:derivation}
%In this Appendix, we derive the main formulas needed for the implementation of the algorithm.

Consider the heterogeneous outer-built Koch snowflakes built on the equilateral triangle with length $L$, while the generator is related to parameter $r$ such that the coefficient reads $c_r = 2(1+r\sin\frac{\Theta}{2})$. 
For the sake of simplicity, we denote a segment sign sequence as $\{s\} = \{ - + \cdots + \}$, in which only the first sign is minus and all the rest (whose number depends on the subscript generation) is plus. Then some typical areas of triangle can be expressed as below:  
\begin{equation} \begin{align}
A_{\Theta,g-1}^{\{s\}} &= \llp \ell_{\Theta,g-1}^{\{s\}} \rrp^2 \frac{\sin\Theta}{2} = \llp \frac{r L}{c_r^{g-1}} \rrp^2 \frac{\sin\Theta}{2} \,, \\
%A_{g}^{\{s\}} &= \llp \ell_{g}^{\{s\}} \rrp^2 \frac{\sin\Theta}{2} = \llp \frac{r L}{c_r^{g}} \rrp^2 \frac{\sin\Theta}{2} \,, \\
A_{\Theta,g}^{\{s-\}} &= \llp \ell_{\Theta,g}^{\{s-\}} \rrp^2 \frac{\sin\Theta}{2} = \llp \frac{r^2 L}{c_r^{g}} \rrp^2 \frac{\sin\Theta}{2} \,. 
\end{align} \end{equation}




\paragraph{Period} Consider all triangles attached on $A_{\Theta,g}^{\{s\}}$ and the total area $\mathcal{A}_{\Theta,g}^{\{s\}}$ reads
\begin{equation} \begin{align}
\mathcal{A}_{\Theta,g}^{\{s\}} =& A_{\Theta,g}^{\{s\}} + 2 A_{\Theta,g+1}^{\{s-\}} + 4 \llp A_{\Theta,g+2}^{\{s--\}} + A_{\Theta,g+2}^{\{s+-\}} \rrp \\
&+ 8 \llp A_{\Theta,g+3}^{\{s++-\}} + A_{\Theta,g+3}^{\{s+--\}} + A_{\Theta,g+3}^{\{s-+-\}} + A_{\Theta,g+3}^{\{s---\}} \rrp \\
&+ \cdots \\
%=& \llp \ell_{g}^{\{s\}} \rrp^2 \frac{\sin\Theta}{2} + \llp \ell_{g+1}^{\{s-\}} \rrp^2 \sin\Theta + \cdots \\
=& \llp \ell_{\Theta,g}^{\{s\}} \rrp^2 \frac{\sin\Theta}{2} + \llp \frac{r \ell_{\Theta,g}^{\{s\}}}{c_r} \rrp^2 \sin\Theta \\
&+ \lls \llp \frac{r^2 \ell_{\Theta,g}^{\{s\}}}{c_r^2} \rrp^2 + \llp \frac{r \ell_{\Theta,g}^{\{s\}} }{c_r^2} \rrp^2 \rrs (2\sin\Theta) + \cdots \\
=& A_{\Theta,g}^{\{s\}} +  \sin\Theta \sum_{i=0}^\infty 2^i \llc \sum_{j=0}^i \lls \mathrm{C}^j_i \llp \frac{r^{j+1} \ell_{\Theta,g}^{\{s\}}}{c_r^{i+1}} \rrp^2  \rrs \rrc \\
=& \llp \ell_{g}^{\{s\}} \rrp^2 \frac{\sin\Theta}{2} + \sin\Theta \frac{\llp r \ell_{g}^{\{s\}} \rrp^2}{c_r^2 - 2(1+r^2)} \,. 
\end{align} \end{equation}
Recall that the binomial coefficient is $\mathrm{C}^j_i = \frac{i!}{j! (i-j)!}$ and $0! = 1$. 
Note, the second summation is simplified by the binomial theorem, and then the whole expression is converted to a geometric progression for the final result.  
%%
If we take $r=1$ for normal Koch snowflakes, we recover Eq. (\ref{eq:Aast}) as $c_1 = 2(1+\sin\frac{\Theta}{2})$ and $\ell_{g}^{\{s\}} \to \ell_{\Theta,g}$. 


\begin{comment}
\begin{equation} \begin{aligned}
\mathcal{A}_{\Theta,g}^\ast %&= A_{\Theta,g} + 2 A_{\Theta,g+1} + 8 A_{\Theta,g+2} + \cdots \\
&= A_{\Theta,g} + 2 \sum_{i=0}^n 4^i A_{\Theta,g+1+i} \\
&= \frac{\ell_{\Theta,g}^2 \sin\Theta}{2} + \frac{\ell_{\Theta,g}^2 \sin\Theta}{(2[1+\sin(\Theta/2)])^2 - 4} \,.
\end{aligned} \end{equation}

\begin{equation} \frac{\mathcal{A}^\ast_{\Theta,g-1}}{\mathcal{A}_{\Theta,g}^\ast} = \frac{A_{\Theta,g-1} + 2 \sum_{i=0}^n 4^i A_{\Theta,g+i}}{A_{\Theta,g} + 2 \sum_{i=0}^n 4^i A_{\Theta,g+1+i}} = \frac{A_{\Theta,g-1}}{A_{\Theta,g}} \,. \end{equation}
\end{comment}


\paragraph{Mean value} The equivalent area requires 
\begin{equation} \begin{align}
A_{\Theta,g-1}^{\{s\}} + 2 A_{\Theta,g}^{\{s-\}} &= A_{g-1}^{\{s\}} (\Theta^\prime) \,, \\
h^{\{s\}}_{\Theta,g-1} d_0 + \ell^2_{\Theta,g} \sin\Theta &= h^{\{s\}}_{\Theta,g-1} d \,. 
\end{align} \end{equation} 
%$$ d = d_0 + \frac{\ell^2_{\Theta,g} \sin\Theta}{h_{\Theta,g}} \,. $$
%$$ d = d_0 + \frac{2\ell^2_{\Theta,g}}{h_{\Theta,g}} \sin(\Theta/2) \cos(\Theta/2) \,, $$
Recall that $h^{\{s\}}_{\Theta,g-1} = \ell^{\{s\}}_{\Theta,g-1} \cos\frac{\Theta}{2}$ and $d_0 = \ell^{\{s\}}_{\Theta,g-1} \sin\frac{\Theta}{2}$, $A_{\Theta,g-1}^{\{s\}} = h^{\{s\}}_{\Theta,g-1} d_0$. 
We solve $\Theta^\prime$ by 
\begin{equation} 
\tan \llp \frac{\Theta^\prime}{2} \rrp = \frac{d}{h^{\{s\}}_{\Theta,g-1}} = \frac{d_0}{h^{\{s\}}_{\Theta,g-1}} + \llp \frac{\ell^{\{s\}}_{\Theta,g}}{h^{\{s\}}_{\Theta,g-1}} \rrp^2 \sin\Theta  \,, 
\end{equation}
and then the effective mean LPE $\bar{\alpha}^\mrm{eff}_\Theta$ in Eq. (\ref{eq:meanvr}) by
\begin{equation} \begin{align}
\bar{\alpha}^\mrm{eff}_\Theta &= \frac{\pi}{2 \Theta^\prime} = \frac{\pi}{4\arctan(d/h^{\{s\}}_{\Theta,g-1})} \,. \\
%&= \frac{\pi}{4\arctan \lls \tan \frac{\Theta}{2} \llp 1 + \frac{2 r^2}{c_r^2} \rrp \rrs }
\end{align} \end{equation}
Eq. (\ref{eq:meanalpha}) is recovered if we set $r = 1$. 
\begin{comment}
$$ \begin{align}
\bar\alpha^\mrm{eff}_\Theta &= \frac{\pi}{2\Theta^\prime} = \frac{\pi}{ 4\arctan(d/h)} \\
&= \frac{\pi}{4\arctan \llc \tan\frac{\Theta}{2} \lls 1 + \frac{1}{2 \llp 1 + \sin \frac{\Theta}{2} \rrp^2} \rrs \rrc} \,. 
\end{align} $$
$$ A_{g-1}^{\{s\}} + 2 A_g^{\{s-\}} = \frac{\sin\Theta}{2} \llp \ell^{\{s\}}_{g-1} \rrp^2 + \llp \frac{r \ell^{\{s\}}_{g-1}}{c_r} \rrp^2 \sin\Theta $$
\end{comment}
